# Supplementary material for: Technical Report: Full Version of Analyzing and Optimizing Perturbation of DP-SGD Geometrically
Source: arXiv:2504.05618 source file (2025-04-08)
Supplement: Supplementary file 1 [file appendix.tex]

\section{Tables}
\begin{table}[h!]
	\centering
	\caption{Parameters for Logistic Regression on MNIST}
	\label{tab::LR}
	\begin{tabular}{c|c|c|c}
		\hline
		Layer & Weights & Biases & Total \\ \hline
		Output (10 classes) & $784 \times 10 = 7840$ & $1 \times 10 = 10$ & 7850 \\ \hline
	\end{tabular}
\end{table}

\begin{table}[ht]
	\centering
	\caption{MLP Architecture and Parameters on CIFAR-10.}	
	\label{tab::MLP}
	\begin{tabular}{@{}llr@{}}
		\toprule
		Layer & Description & Number of Parameters \\
		\midrule
		Input       & 3072 dimensions (32x32x3) & 0 \\
		Hidden      & 200 neurons, tanh activation & $(3072 + 1) \times 200 = 614,\!600$ \\
		Output      & 10 classes (CIFAR-10) & $(200 + 1) \times 10 = 2,\!010$ \\
		\midrule
		Total       & & $614,\!600 + 2,\!010 = 616,\!610$ \\
		\bottomrule
	\end{tabular}
\end{table}
